# Supplementary material for: DRL-Based Trajectory Tracking for Motion-Related Modules in Autonomous Driving
Source: arXiv:2308.15991 source file (2024-03-24)
Supplement: Supplementary file 1 [file appendix.tex]

% Appendixes should appear before the acknowledgment.
% \setcounter{subsection}{0}

% \subsection{Environment \& training details}
% \label{subsec:environment-and-training-details}

% In this section, we present the implementation details of our DRL learning algorithm in Table~\ref{tab:env-rl-hyperparams}. We use the Multi-Layer Perceptron (MLP)~\cite{haykin1998neural} to build the policy network (actor) and the value network (critic). Their architectures are described by hidden layer dimensions.

% \input{body/assets/table-env-rl-hyperparams.tex}




% \subsection{Dynamics model details}
% \label{subsec:dynamics-model-details}
% % TODO: refine this part

% \input{body/assets/table-dynamics-model-definitions}

% For the \textit{vehicle} and the \textit{cyclist} categories, we use the single-track bicycle model~\cite{rajamani2011vehicle}:
% % https://archit-rstg.medium.com/two-to-four-bicycle-model-for-car-898063e87074
% \begin{equation}
% \begin{array}{rl}
%     \dot{x} &= v \cdot \cos\left( \theta + \beta \right) \\
%     \dot{y} &= v \cdot \sin\left( \theta + \beta \right) \\
%     \dot{\theta} &= \frac{v \cdot \sin\left( \delta \right)}{L} \\ 
%     \dot{v} &= a \\
%     \beta &= \arctan\left( \frac{l_r}{l_f+l_r} \tan\left( \delta \right) \right) \\ 
%     L &= l_f + l_r \\
% \end{array}
% \end{equation}
% where the state variables $x$, $y$, $\theta$, and $v$ denote the X-coordinate, the Y-coordinate, the heading, and the scalar speed of the Center of Mass (CoM), respectively. $\beta$ is the difference between the speed direction of CoM and the vehicle heading, and $l_f$ and $l_r$ are distances from the CoM to the front and the rear axle, respectively. $L$ is the wheelbase.

% To model dynamics for the \textit{pedestrian} category whose motion pattern has a higher degree of freedom, we use the unicycle model~\cite{batkovic2018computationally, karasev2016intent},
% \begin{equation}
% \begin{array}{rl}
%     \dot{x} &= v \cdot \cos\left( \theta \right) \\
%     \dot{y} &= v \cdot \sin\left( \theta \right) \\
%     \dot{\theta} &= \omega \\
%     \dot{v} &= a \\
% \end{array}
% \end{equation}
% where $\omega$ is the heading change rate. The notation for other variables remains the same as in the bicycle model.



% \subsection{Hyper-parameters of dynamics models}
% \label{subsec:hyper-parameters-of-dynamics-models}

% While the distribution $\mathcal{D}_{\theta_d}$ can be any desired continuous/discrete distribution of the parameters of the dynamics model, we use a discrete uniform distribution (i.e. all combinations have an equal probability to be sampled) for our demonstration experiment within this work. Table~\ref{tab:dynamics-model-parameters} lists all possible parameter combinations.

% \input{body/assets/table-dynamics-model-parameters.tex}
